# Supplementary material for: Experimental Design in Two-Sided Platforms: An Analysis of Bias
Source: arXiv:2002.05670 source file (2021-09-26)
Supplement: Supplementary file 1 [file appendix_bias_example.tex]

\label{app:bias_examples}

In the remainder of the paper, we study the behavior of the $\CR$, $\LR$, and $\TSR$ designs and associated naive estimators proposed in the previous section.  We are particularly interested in characterizing the {\em bias}: i.e., the extent to which the estimators we have defined under- or overestimate the true $\GTE$.%

In this section, we start with a simple discussion via example that illustrates the main effects that cause bias. 
To simplify the discussion we will assume that there are $N = 2$ listings in total in the market. Further, we assume that listings are homogeneous (i.e., of identical type) and that arriving customers are homogeneous as well (i.e., of identical type).  We let $v > 0$ denote the utility of a customer for a listing, and suppose the platform considers an intervention that changes this utility to $\tilde{v} > 0$.  Finally, we assume that every arriving customer includes any listing that is available in their consideration set, that is, $\alpha=1$.  

An important operational finding of our work is that the {\em market balance} $\lambda/\tau$ has a significant influence in determining which estimator and design is bias-optimal.  When $\lambda/\tau$ becomes large, the market is relatively {\em supply-constrained}: customers are arriving much faster than occupied listings become available.  When $\lambda/\tau$ becomes small, the market is {\em demand-constrained}, with few customers arriving and many available listings.  We divide our discussion of this example into these two extreme cases.  Our findings are illustrative of the insights we obtain theoretically in the next section.

\subsection{Highly demand-constrained markets}

Consider a hypothetical limit where each listing becomes instantly available again after being booked (i.e., $\tau \to \infty$ but $\lambda$ remains fixed).  This is the demand-constrained extreme, where capacity constraints on listings become irrelevant.  Note that on arrival of a customer, both listings are always available, and therefore, included in the consideration set.  In this limit, observe that the steady-state rate at which customers book listing $\ell = 1,2$ becomes:
\begin{equation}
\label{eq:example_rate_dc}
\frac{\lambda v}{\epsilon + 2 v}.
\end{equation}
(The factor 2 appears in the denominator as there are two listings.)  Since the intervention changes $v$ to $\tilde{v}$, the $\GTE$ is:
\[ \GTE = \frac{2 \lambda \tilde{v}}{\epsilon + 2 \tilde{v}} - \frac{2\lambda v}{\epsilon + 2v}. \]

Now suppose we consider a $\CR$ design that randomizes a fraction $a_C$ of arriving customers to treatment.  Observe that in this demand-constrained extreme, every arriving control (resp., treatment) customer sees the full global control (resp., treatment) market condition; there is no dynamic influence of one customer's booking behavior on any other customer.  This suggests the naive $\CR$ estimator should correctly recover the global treatment effect.  Indeed, the steady-state naive $\CR$ estimator becomes:
\[ \widehat{\GTE}^{\CR}(\infty | a_C) = \frac{1}{a_C} \frac{2 a_C \lambda \tilde{v}}{\epsilon + 2 \tilde{v}} - \frac{1}{1-a_C} \frac{2 (1-a_C) \lambda v}{\epsilon + 2 v} = \GTE. \]
In other words, the naive $\CR$ estimator is perfectly {\em unbiased}.  

On the other hand, consider a $\LR$ design where listing 1 is (randomly) assigned to treatment, and listing 2 is (randomly) assigned to control.  In this design, the steady-state naive $\LR$ estimator (with $a_L = 1/2$) becomes:
\[ \widehat{\GTE}^{\LR}(\infty | a_L) =  \frac{1}{a_L} \frac{\lambda \tilde{v}}{\epsilon + v + \tilde{v}} - \frac{1}{1-a_L} \frac{\lambda v}{\epsilon + v + \tilde{v}}. \]
It is clear that in general this will {\em not} be equal to the $\GTE$, because there is {\em interference} between the two listings: {\em every} arriving customer sees a market environment that is neither quite global treatment nor global control, and the estimates reflect this imperfection.  Even with immediate replenishment, treatment listings compete for customers and ``cannibalize" bookings from control listings,
causing the naive $\LR$ estimator to be biased.  (Note that such a violation would arise for virtually any reasonable choice model that could be considered.) 

\subsection{Highly supply-constrained markets}

Now we consider the opposite extreme, where the market is heavily supply constrained; in particular, we consider the hypothetical limit where $\lambda \to \infty$ but $\tau$ remains fixed.  Now in this case, note that a listing that becomes available will {\em nearly instantaneously} be booked; therefore, virtually every arriving customer will find at most one of the two listings available, and their decision of whether to book will be entirely determined by comparison of that available listing against the outside option.  In particular, as a result when $\lambda \to \infty$ the steady-state rate at which listing $\ell = 1,2$ is booked approaches $\tau$.

We thus require a more refined estimate of this booking rate as $\lambda \to \infty$.  Suppose $\lambda$ is large, and suppose listing $\ell$ becomes available.  Based on the intuition above, we make the approximation that the listing will be considered in isolation by a succession of customers until it is booked.  Customers arrive at rate $\lambda$, and book an available listing with probability $v/(\epsilon + v)$; in other words, in this regime listings compete only with the outside option, and not with each other.  Therefore the mean time until such a booking occurs is $(\epsilon + v)/\lambda v$; and once booked, the listing remains booked for mean time $1/\tau$, at which time it becomes available again.  Therefore for large $\lambda$, the long-run average rate at which a listing $\ell = 1,2$ is booked is approximately:
\begin{equation}
\label{eq:example_rate_sc}
\left( \frac{\epsilon + v}{\lambda v} + \frac{1}{\tau}\right)^{-1}.
\end{equation}
As expected, this rate approaches $\tau$ as $\lambda \to \infty$.  The $\GTE$ is thus:
\[ \GTE = 2\left( \frac{\epsilon + \tilde{v}}{\lambda \tilde{v}} + \frac{1}{\tau}\right)^{-1} - 2 \left( \frac{\epsilon + v}{\lambda v} + \frac{1}{\tau}\right)^{-1}. \]

With this observation in hand, suppose we again consider the same $\LR$ design where listing 1 is (randomly) assigned to treatment, and listing 2 is (randomly) assigned to control.  Since in \eqref{eq:example_rate_sc} there is no influence of one listing on the other, observe that the naive $\LR$ estimator (with $a_L = 1/2$) becomes:
\[ \widehat{\GTE}^{\LR}(\infty | a_L) = \frac{1}{a_L} \left( \frac{\epsilon + \tilde{v}}{\lambda \tilde{v}} + \frac{1}{\tau}\right)^{-1} - \frac{1}{1-a_L}\left( \frac{\epsilon + v}{\lambda v} + \frac{1}{\tau}\right)^{-1} = \GTE. \]
In other words, the naive $\LR$ estimator is perfectly {\em unbiased}.  This is intuitive: in the limit where $\lambda$ is large, since listings do not compete with each other for bookings, there is no interference when we implement the $\LR$ design.

On the other hand, consider the naive $\CR$ design where a fraction $a_C$ of arriving customers are randomized to treatment.  In this case we wish to establish the rate at which bookings are made by treatment and control customers respectively.  Suppose listing $\ell$ was occupied by a treatment customer, and becomes available.  Define:
\[ \zeta(a_C) = a_C \tilde{v}/(\epsilon + \tilde{v}) + (1 - a_C)v/(\epsilon + v). \]
This is the probability an arriving customer books the available listing.  Customers arrive at rate $\lambda$, so a mean time $1/(\lambda \zeta(a_C))$ elapses until a booking is made; the listing then remains occupied for mean time $1/\tau$.  Hence, the long-run average rate at which bookings of listing $\ell$ occur is given by $(1/(\lambda \zeta(a_C))+1/\tau)^{-1}$. 
Now, conditional on a booking, the booking was made by a treatment customer with probability:
\[ \eta(a_C) = \frac{1}{\zeta(a_C)} \frac{a_C \tilde{v}}{\epsilon + \tilde{v}}. \]
Hence, 
Thus the long-run average rate at which listing $\ell$ is booked by treatment customers is:
\[ \eta(a_C) \cdot \left(\frac{1}{\lambda \zeta(a_C)} + \frac{1}{\tau}\right)^{-1} =  \left( \frac{\epsilon + \tilde{v}}{a_C \lambda \tilde{v}} + \frac{1}{\eta(a_C) \tau} \right)^{-1}. \] 
We can use the same logic for the booking rate of control customers, and so we find the naive $\CR$ estimator is:
\[ \widehat{\GTE}^{\CR}(\infty | a_C) = 
\frac{2}{a_C} \left( \frac{\epsilon + \tilde{v}}{a_C \lambda \tilde{v}} + \frac{1}{\eta(a_C) \tau}\right)^{-1} - 
\frac{2}{1-a_C}\left( \frac{\epsilon + v}{(1-a_C)\lambda v} + \frac{1}{(1 - \eta(a_C))\tau}\right)^{-1}. \]

In general, this estimator will be {\em biased}, i.e., not equal to $\GTE$.  The issue is that in this case, customers have a {\em dynamic} influence on each other across the treatment groups: when a listing becomes available, whether or not it is available for booking by a subsequent control customer depends on whether or not a treatment customer had previously booked the listing. In this case, customers compete among each other for listings. This interference across customer groups leads to the biased expression for the naive $\CR$ estimator.

We note that the $\GTE$ and naive $\LR$ estimators converge to zero in the limit where $\lambda \to \infty$; this is because the booking rate of each listing becomes $\tau$ in this limit.  The naive $\CR$ estimator does {\em not} converge to zero in general, however, as $\lambda \to \infty$, because in general 
$\eta(a_C) = (1/\zeta(a_C)) \cdot (a_C \tilde{v})/(\epsilon + \tilde{v}) \neq  (1/\zeta(a_C)) \cdot ((1-a_C) {v})/(\epsilon + {v}) = 1-\eta(a_C)$.  For example, if $\tilde{v} > v$ and $a_C = 1/2$, these expressions reveal that treatment customers book more often than control customers.

\subsection{Discussion: Violation of SUTVA}

Our simple example illustrates that the naive $\LR$ estimator is biased when $\lambda \to 0$, and unbiased when $\lambda \to \infty$; and the naive $\CR$ estimator is unbiased when $\lambda \to 0$, while it is biased when $\lambda \to \infty$.
These findings can be interpreted through the lens of the classical potential outcomes model; an important result from this literature is that when the {\em stable unit treatment value assumption} (SUTVA) holds, then naive estimators of the sort we consider will be unbiased for the true treatment effect.  SUTVA requires that the treatment condition of units other than a given customer or listing should not influence the potential outcomes of that given customer or listing.  The discussion above illustrates that in the limit where $\lambda \to 0$, there is no interference across customers in the $\CR$ design; this is why the naive $\CR$ estimator is unbiased.  Similarly, in the limit where $\lambda \to \infty$, there is no interference across listings in the $\LR$ design; this is why the naive $\LR$ estimator is unbiased.  On the other hand, the cases where each estimator is biased involve interference across experimental units.
